# Supplementary material for: Constraining the thermally-pulsing asymptotic giant branch phase with resolved stellar populations in the Small Magellanic Cloud
Source: arXiv:1903.04499 ancillary file (2019-03-11)
Supplement: Supplementary file 1 [file appendixC_online.pdf]

## APPENDIX C: OBSERVED AND SIMULATED LUMINOSITY FUNCTIONS

We show here the $K_s$-band luminosity functions computed for each set of models, as compared to the observations, for the entire AGB sample and for the three classes of O-rich, C-rich and X-AGB stars (Figs. C1 – C34). The reader should refer to Sect. 4 for a description of the calculated models (see also Table 4) and their performance (see also Fig. 8 and Table 5).

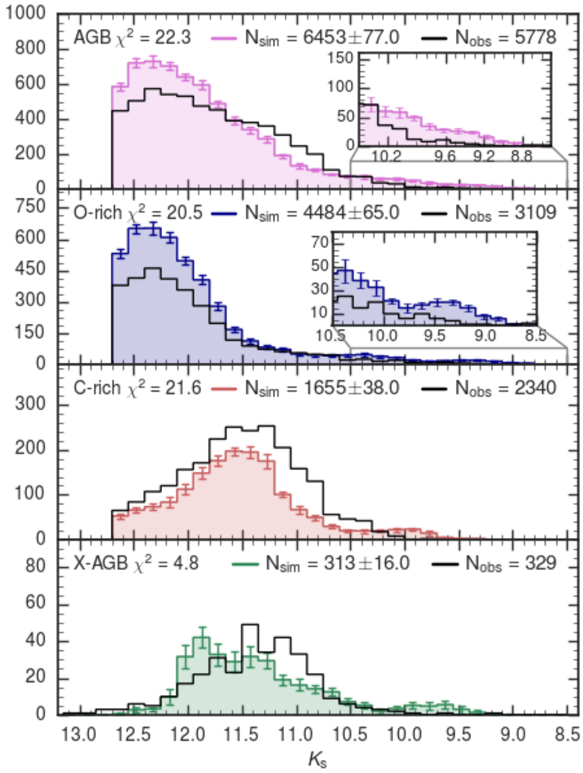


**Figure C1.** $K_s$-band LFs from S_00.

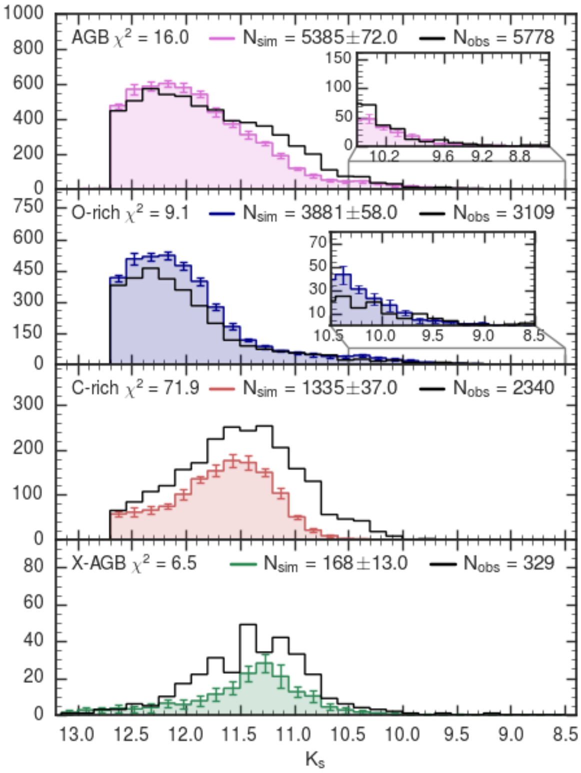


**Figure C2.** $K_s$-band LFs from S_01.

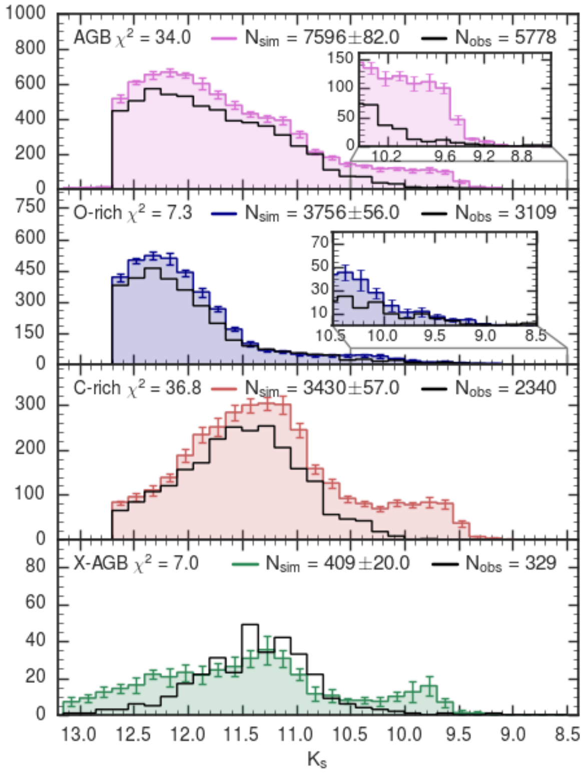


**Figure C3.** $K_s$-band LFs from S_02.

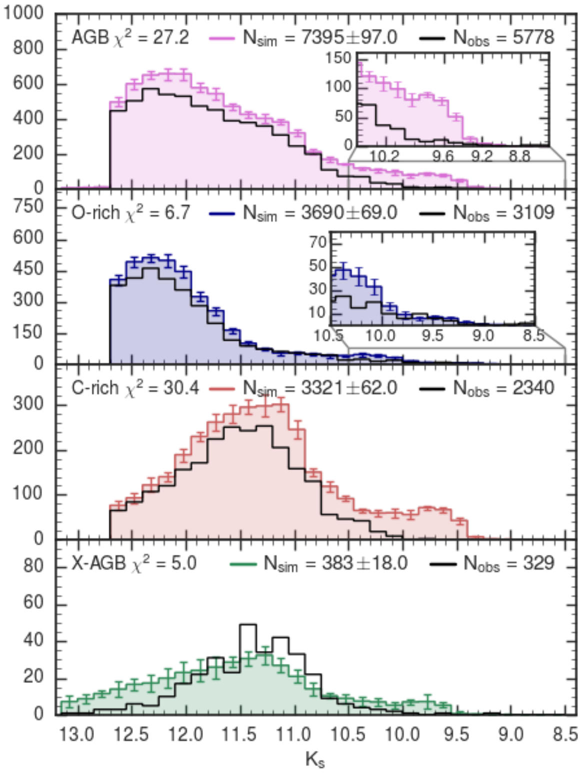


**Figure C4.** $K_s$-band LFs from S_03.

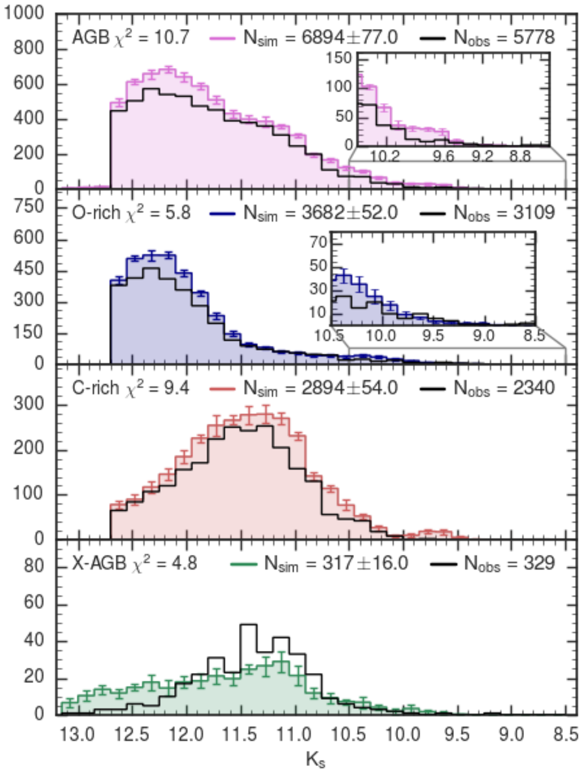


**Figure C5.** $K_s$-band LFs from S_04.

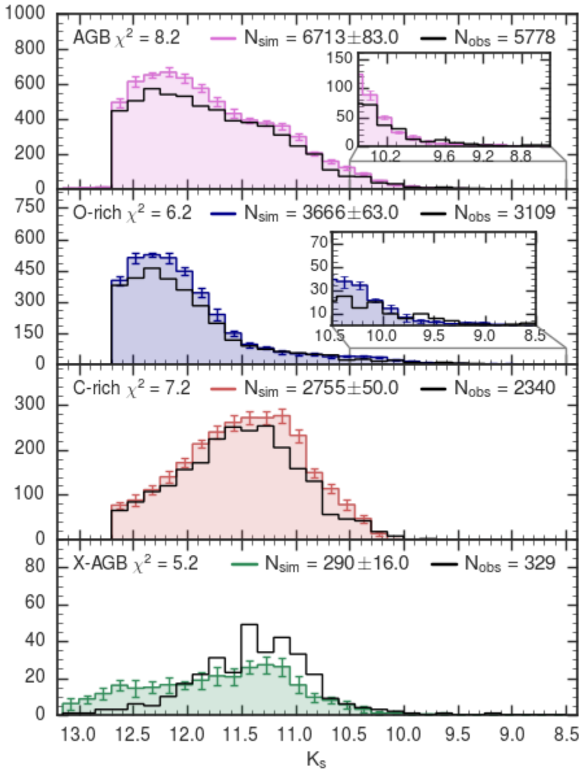


**Figure C6.** $K_s$-band LFs from S_05.

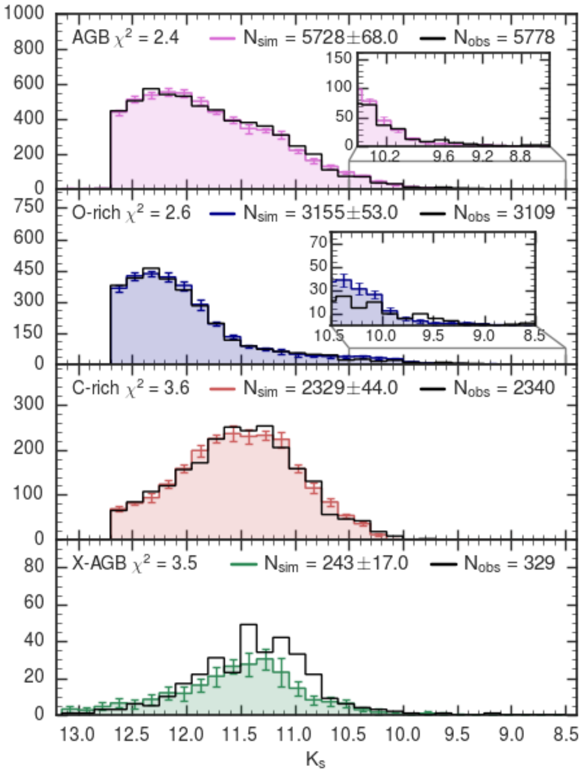


**Figure C7.** $K_s$-band LFs from S_06.

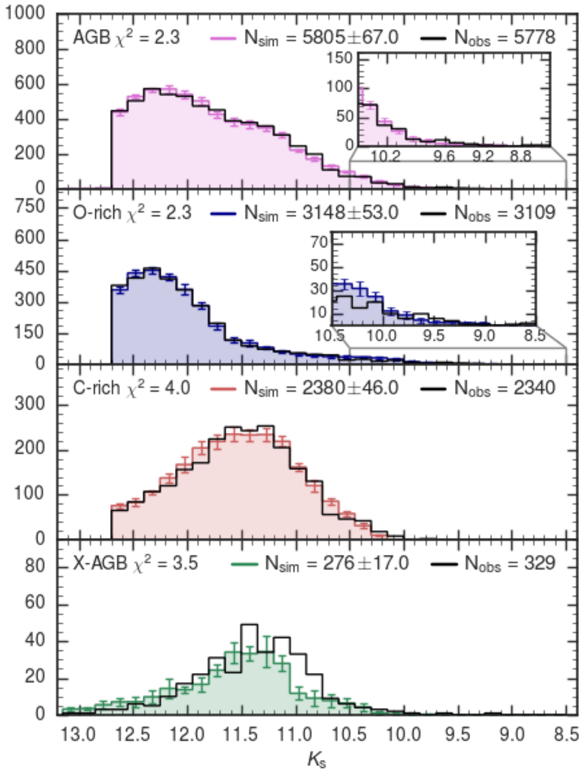


**Figure C8.** $K_s$-band LFs from S_07.

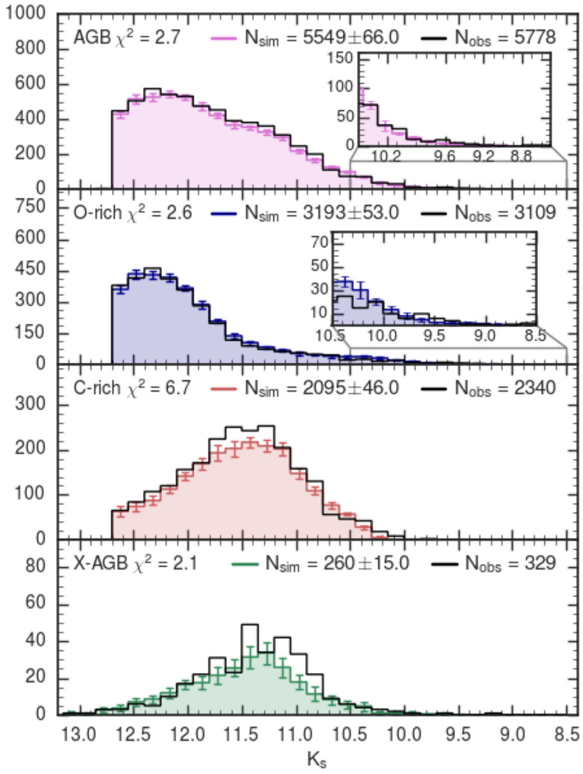


**Figure C9.** $K_S$-band LFs from S_08.

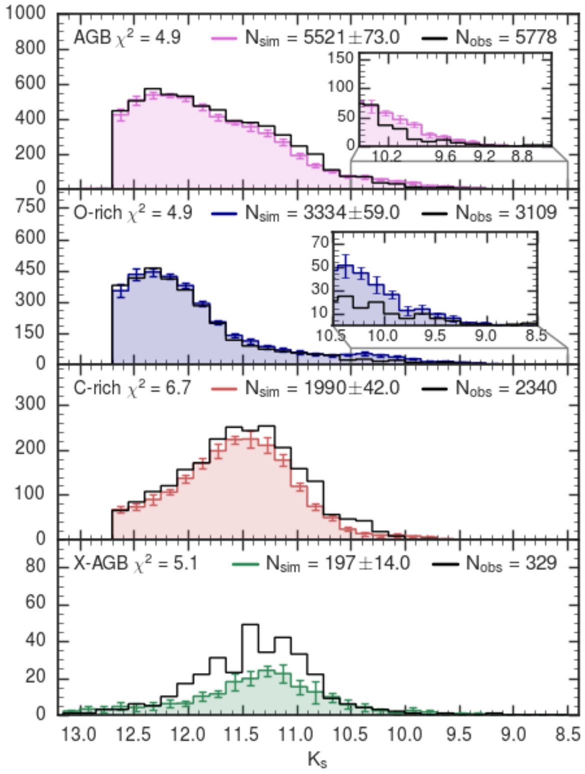


**Figure C10.** $K_S$-band LFs from S_09.

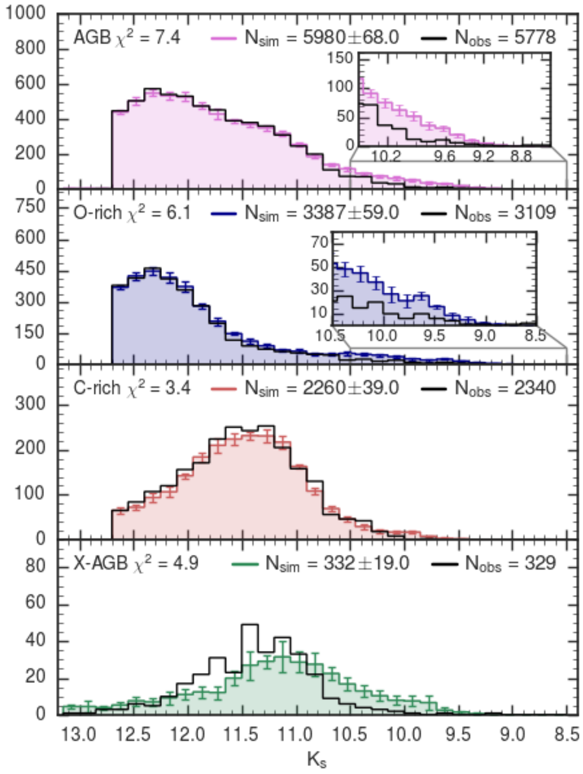


**Figure C11.** $K_S$-band LFs from S_10.

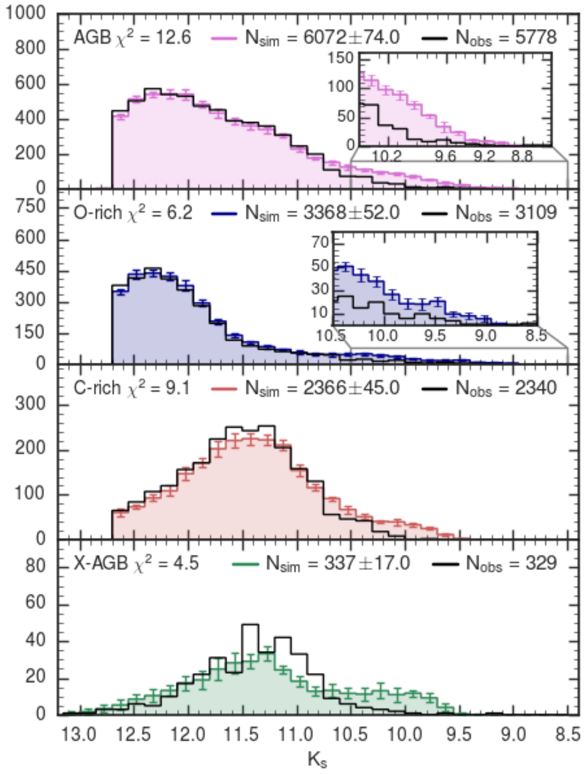


**Figure C12.** $K_S$-band LFs from S_11.

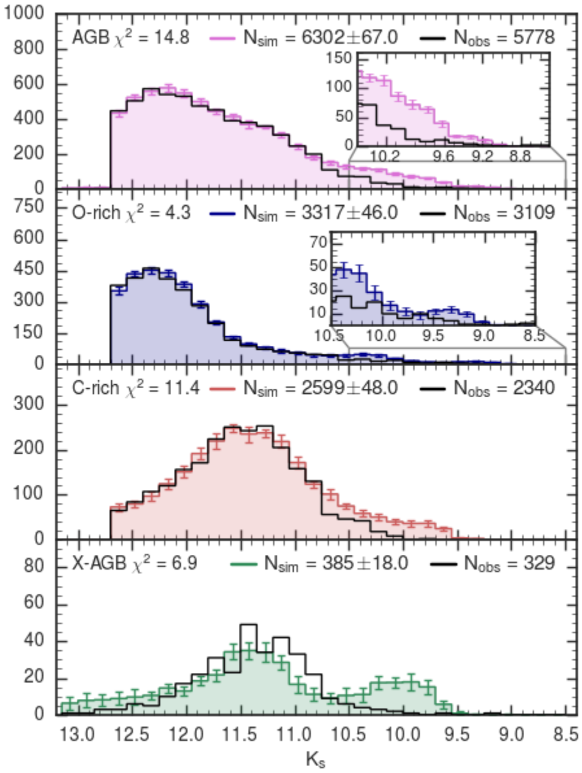


**Figure C13.** $K_\mathrm{s}$-band LFs from S_12.

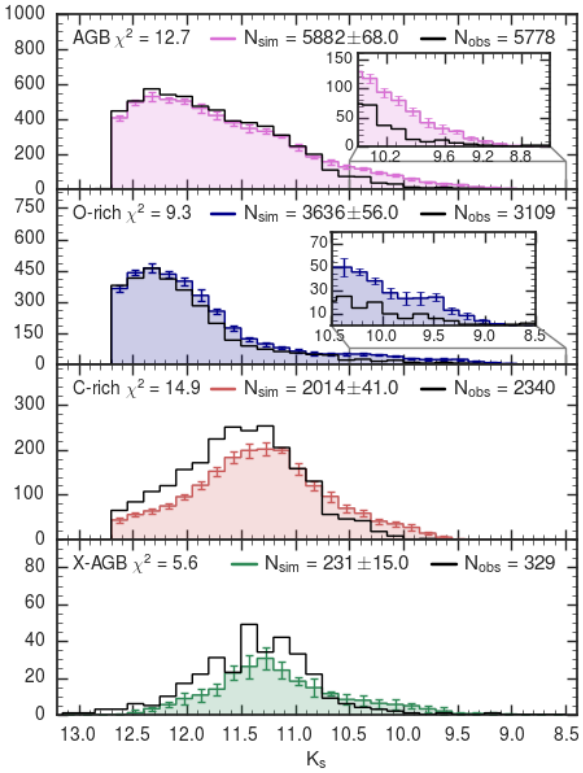


**Figure C14.** $K_\mathrm{s}$-band LFs from S_13.

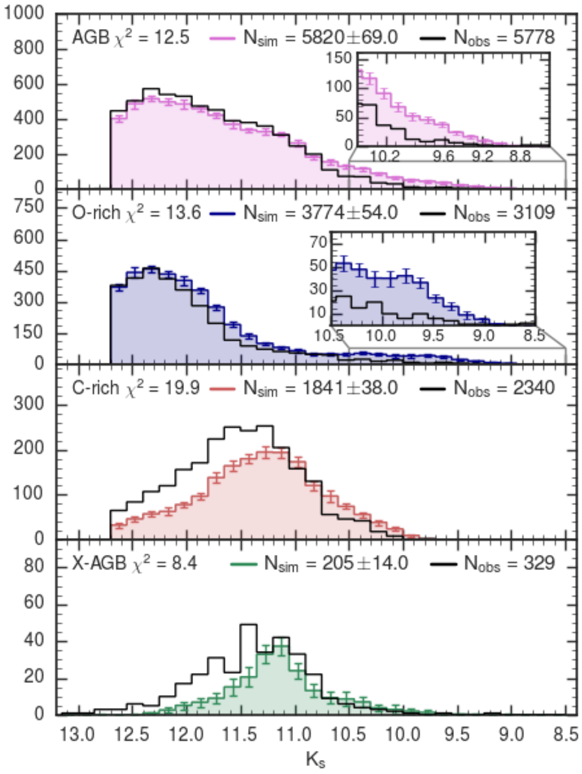


**Figure C15.** $K_\mathrm{s}$-band LFs from S_14.

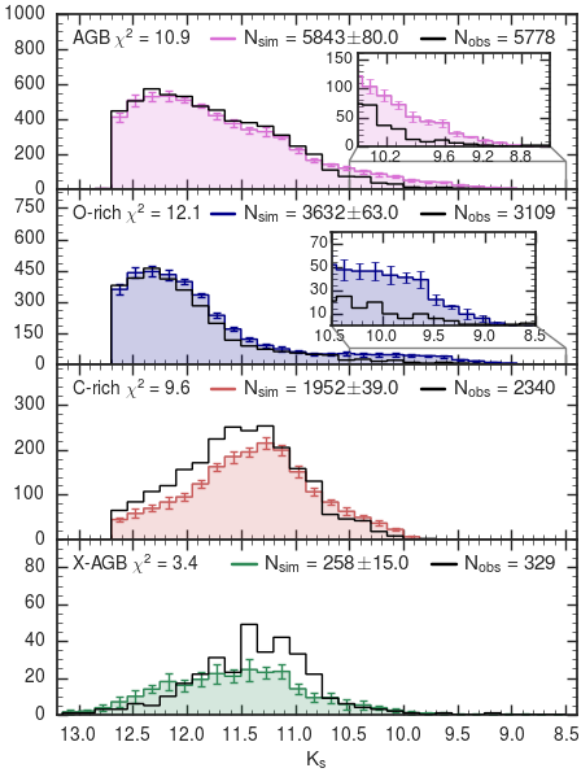


**Figure C16.** $K_\mathrm{s}$-band LFs from S_15.

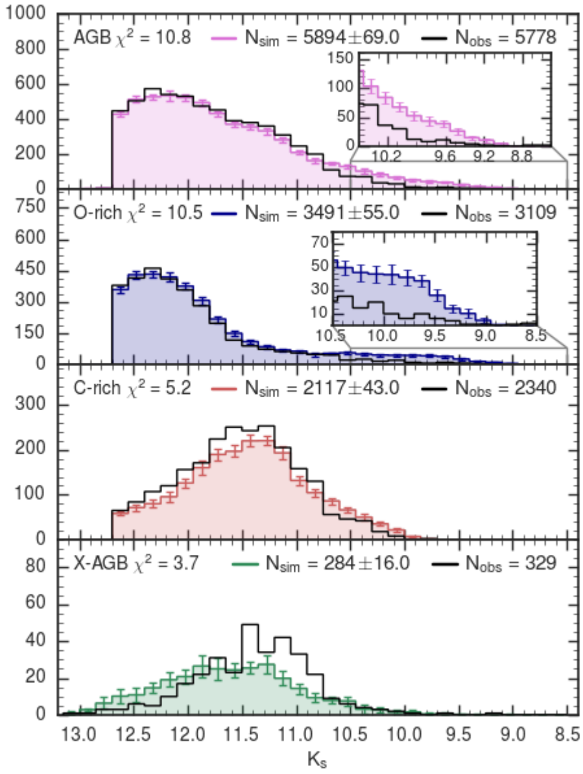


**Figure C17.** $K_{\rm s}$-band LFs from S_16.

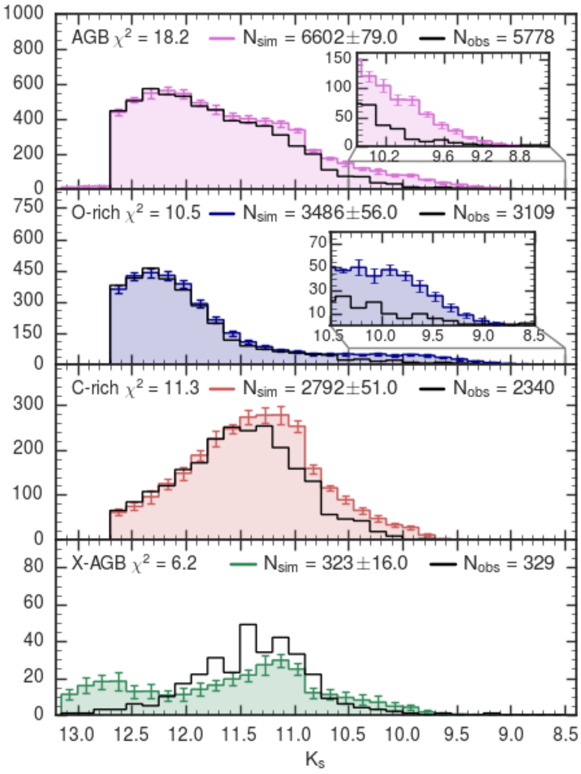


**Figure C18.** $K_{\rm s}$-band LFs from S_17.

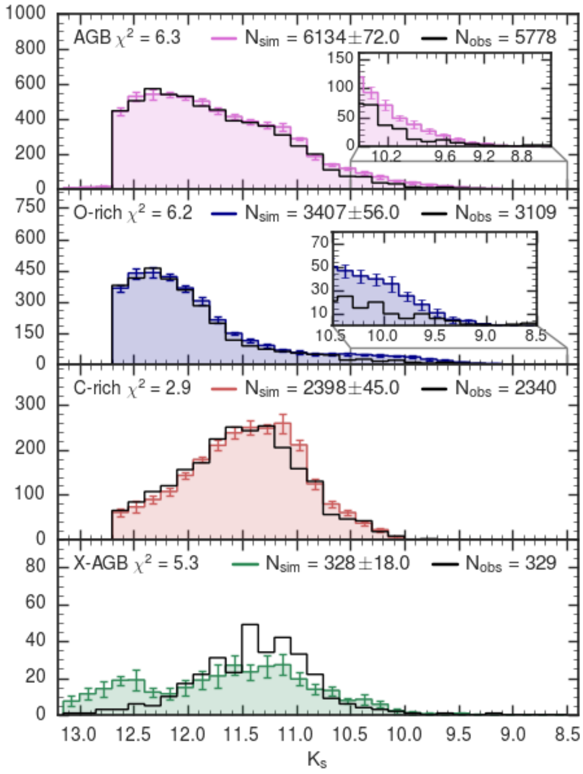


**Figure C19.** $K_{\rm s}$-band LFs from S_18.

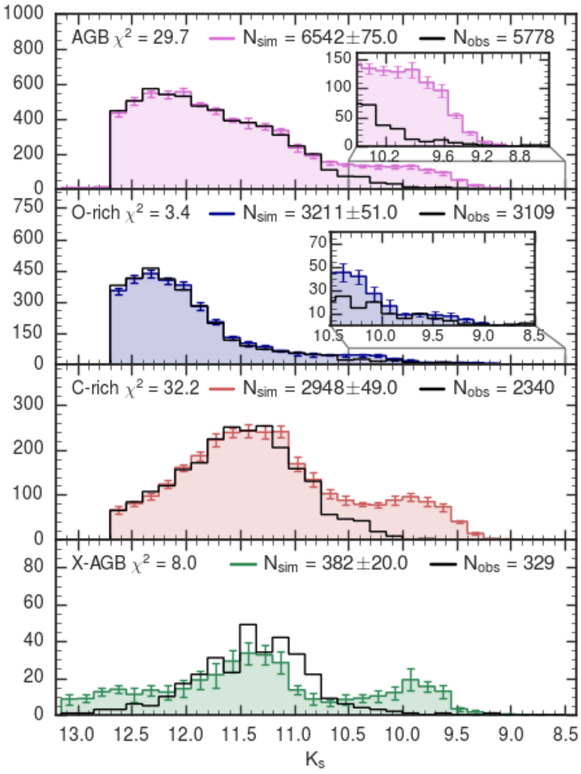


**Figure C20.** $K_{\rm s}$-band LFs from S_19.

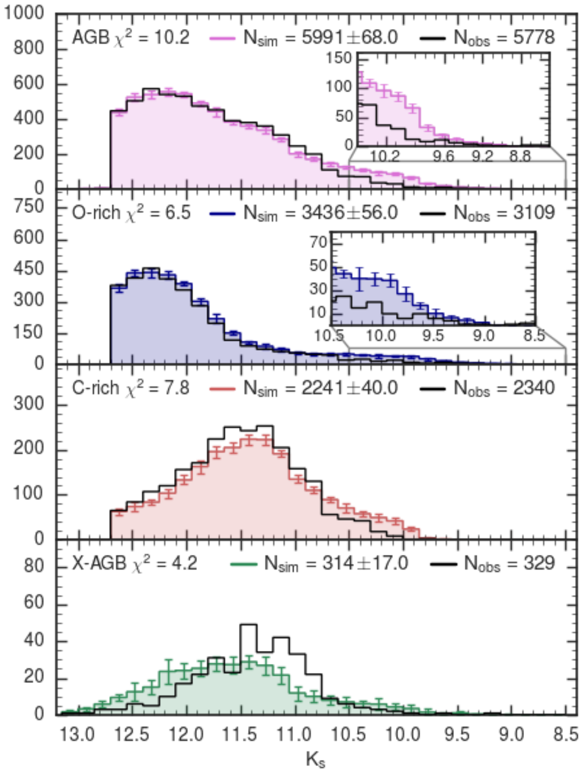


**Figure C21.** $K_S$-band LFs from S_20.

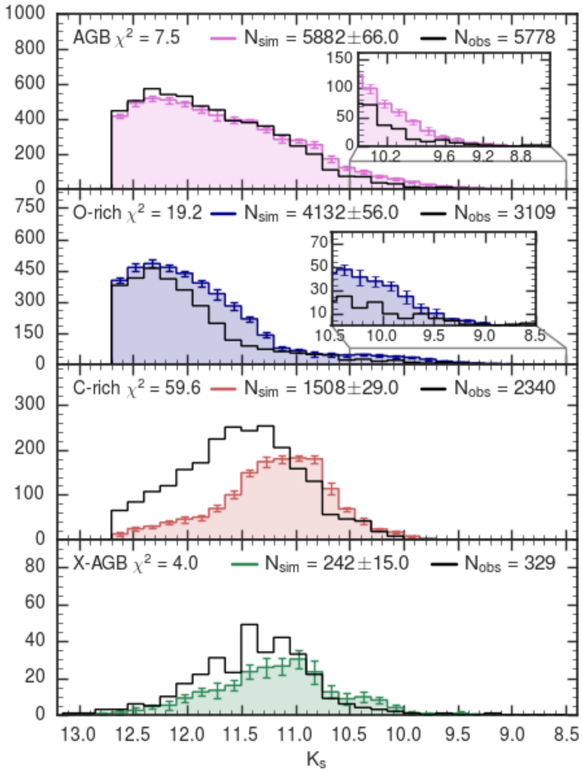


**Figure C22.** $K_S$-band LFs from S_22.

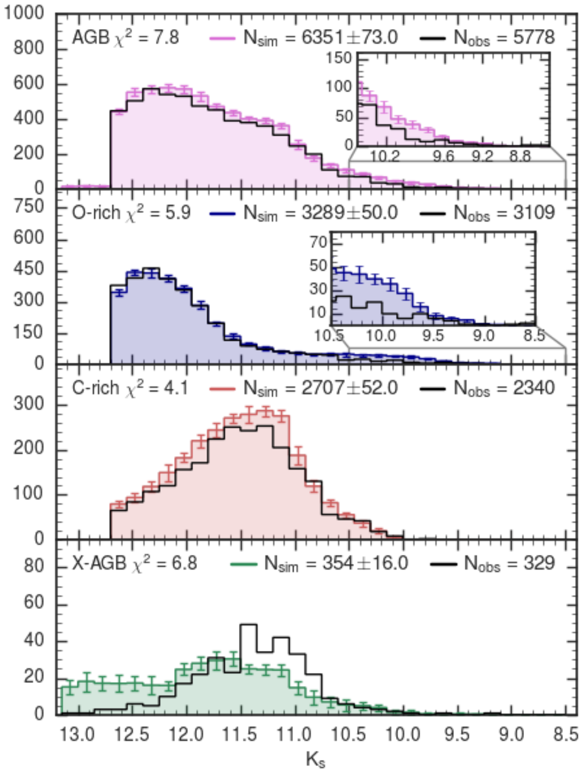


**Figure C23.** $K_S$-band LFs from S_23.

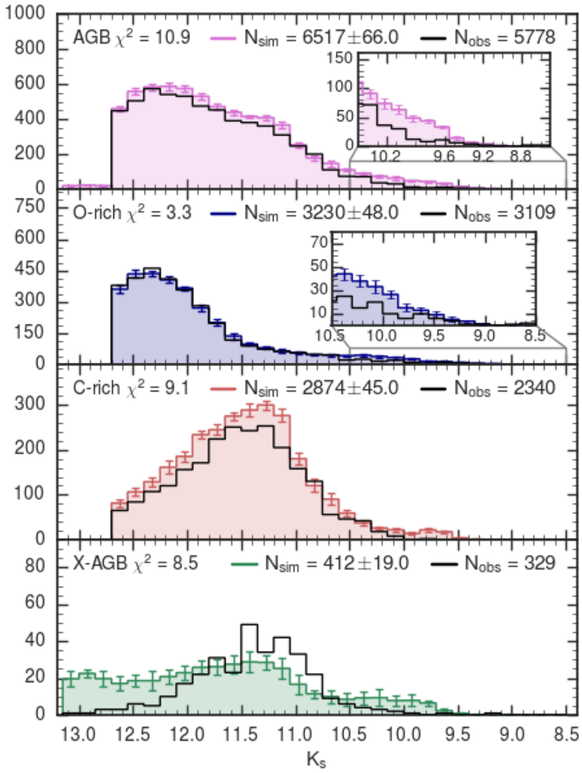


**Figure C24.** $K_S$-band LFs from S_24.

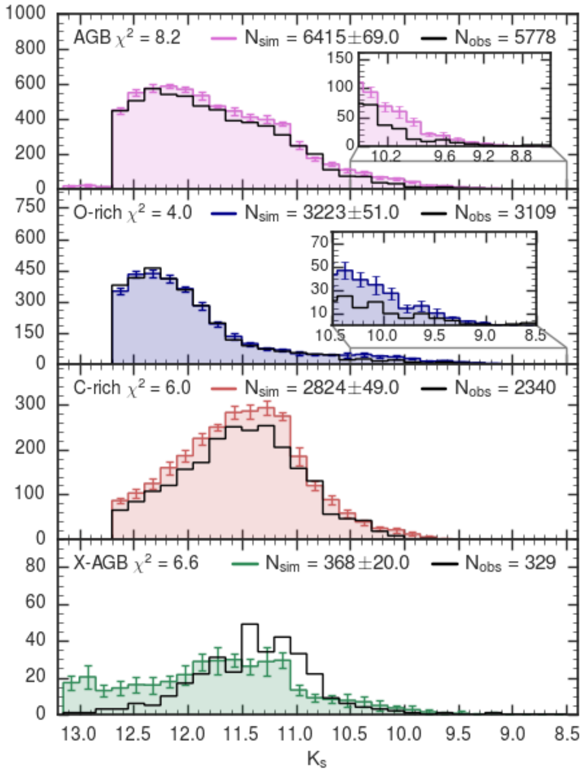


**Figure C25.** $K_\mathrm{S}$-band LFs from S_25.

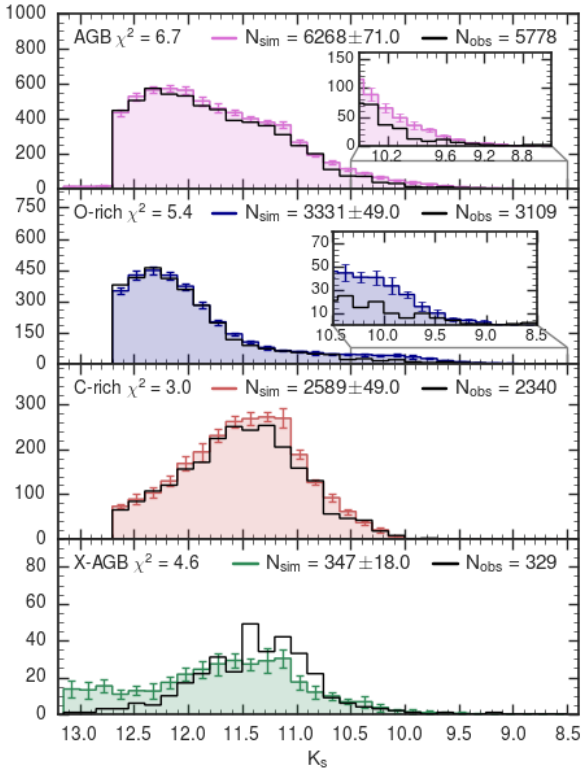


**Figure C26.** $K_\mathrm{S}$-band LFs from S_26.

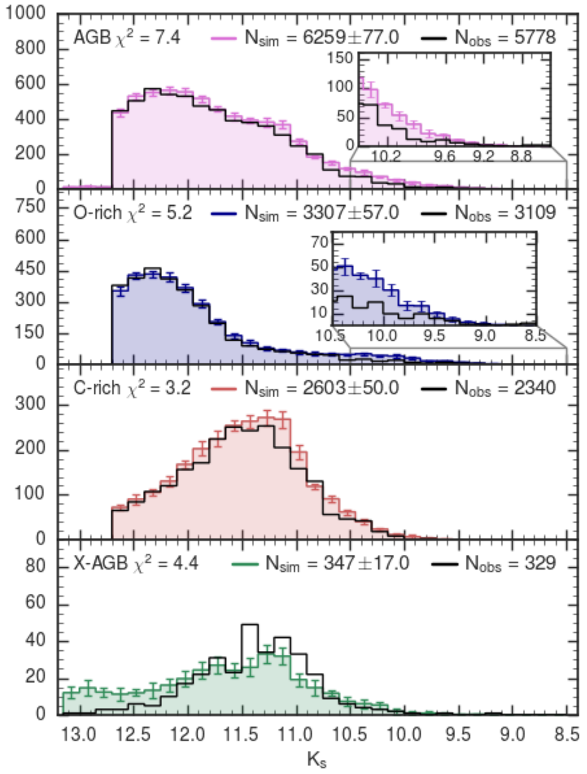


**Figure C27.** $K_\mathrm{S}$-band LFs from S_27.

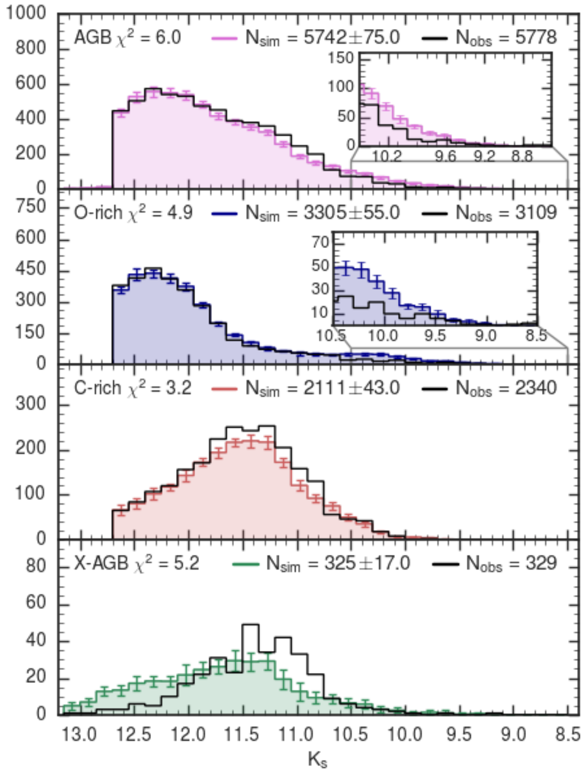


**Figure C28.** $K_\mathrm{S}$-band LFs from S_28.

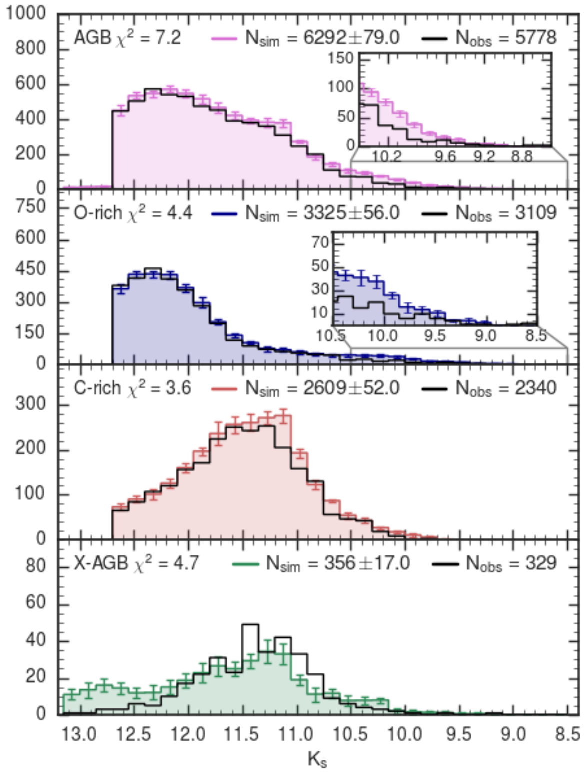


**Figure C29.** $K_s$-band LFs from S_29.

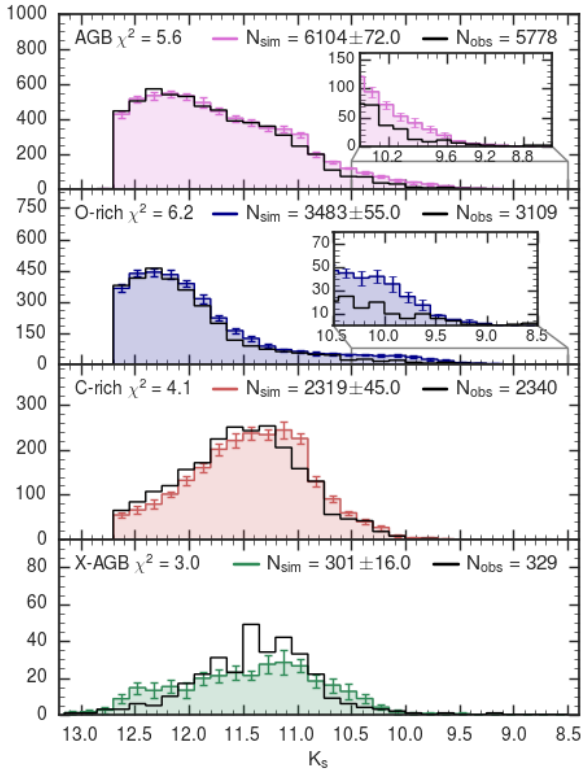


**Figure C30.** $K_s$-band LFs from S_30.

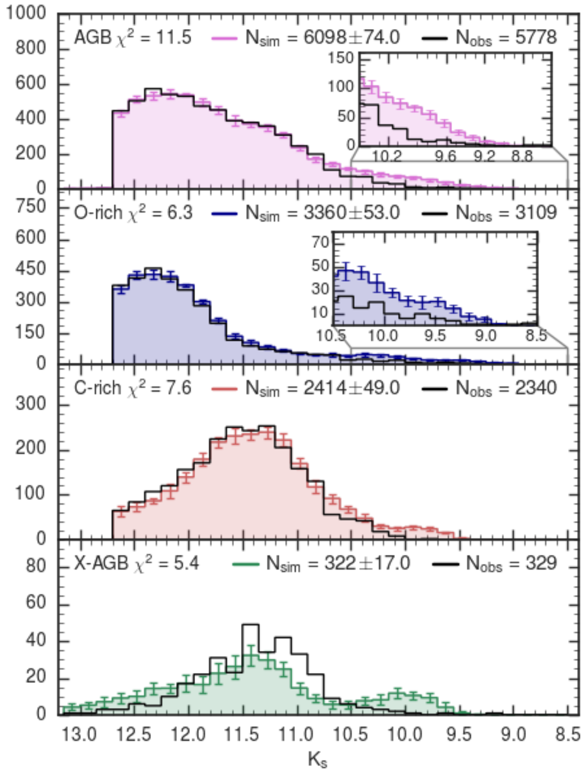


**Figure C31.** $K_s$-band LFs from S_31.

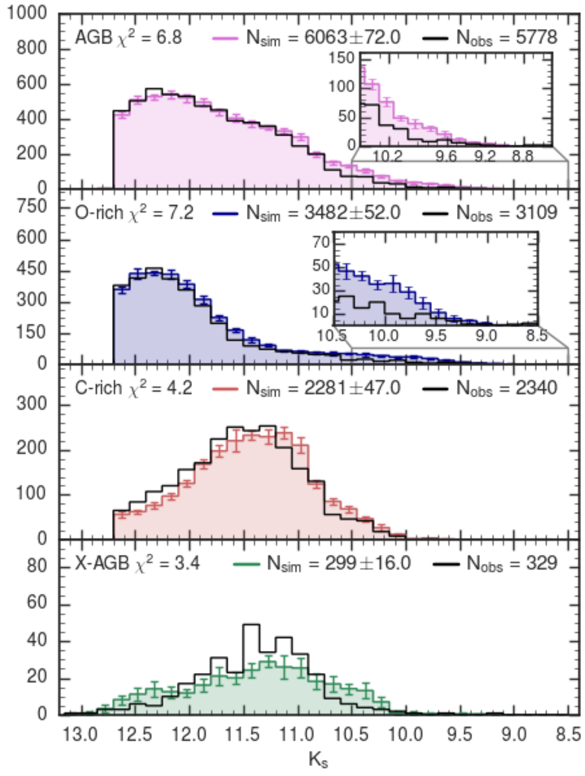


**Figure C32.** $K_s$-band LFs from S_32.

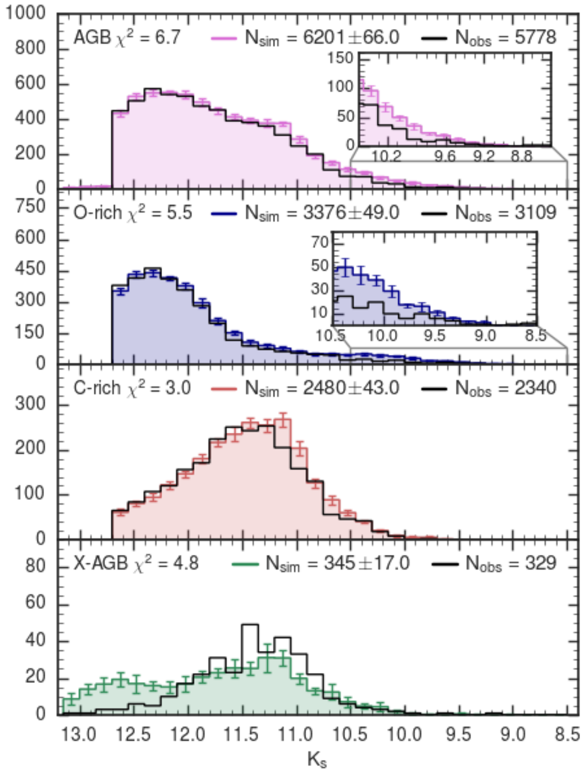


**Figure C33.** $K_{\rm s}$-band LFs from S_34.

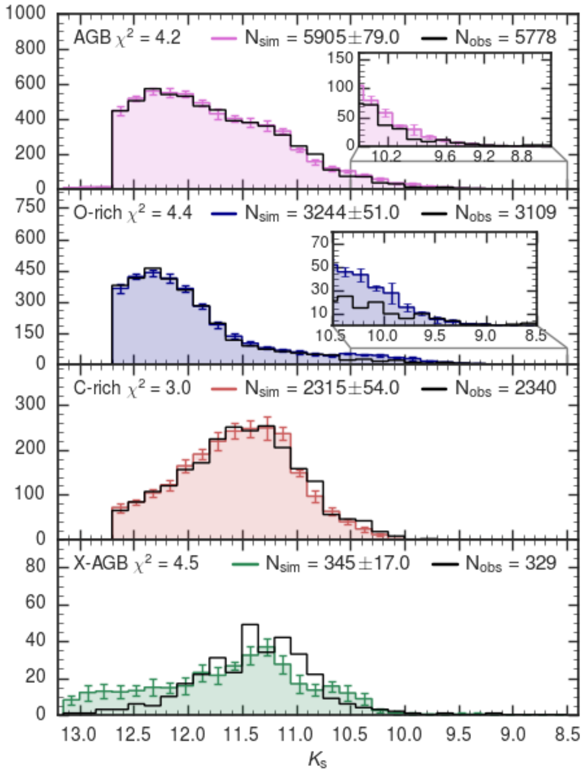


**Figure C34.** $K_{\rm s}$-band LFs from S_35.
